# Supplementary material for: Question Answering for Complex Electronic Health Records Database using Unified Encoder-Decoder Architecture
Source: arXiv:2111.14703 source file (2021-11-14)
Supplement: Supplementary file 1 [file appendix_biomedical_plms.tex]

% \begin{table}[h]
% \vspace{-4mm}
% \centering
% % \resizebox{\columnwidth}{%
% \scriptsize
% \begin{tabular}{llll}
% \hline
% \multirow{2}{*}{\textbf{Method}} &
%   \multicolumn{3}{c}{\textbf{Testing}} \\
%  &
%   \multicolumn{1}{c}{$Acc_{LF}$} &
%   \multicolumn{1}{c}{$Acc_{EX}$} &
%   \multicolumn{1}{c}{$Acc_{ST}$}  \\ \hline
% UniQA$_{BioBERT}$ &
%   $0.852\ {\scriptstyle (0.006)}$ &
%   $0.895\ {\scriptstyle (0.005)}$ &
%   $\textbf{0.900}\ {\scriptstyle (0.005)}$ 
%   \\
% UniQA$_{BlueBERT}$ &
%   $0.852\ {\scriptstyle (0.011)}$ &
%   $0.882\ {\scriptstyle (0.013)}$ &
%   $0.887\ {\scriptstyle (0.011)}$ 
%   \\
% UniQA$_{BERT}$ &
%   $\textbf{0.853}\ {\scriptstyle (0.007)}$ &
%   $\textbf{0.897}\ {\scriptstyle (0.006)}$ &
%   $0.891\ {\scriptstyle (0.009)}$ 
%   \\ \hline
% \textbf{After Recovering} \\
% UniQA$_{BioBERT}$ &
%   $0.000\ {\scriptstyle (0.000)}$ &
%   $0.000\ {\scriptstyle (0.000)}$ &
%   $0.000\ {\scriptstyle (0.000)}$ 
%   \\
% UniQA$_{BlueBERT}$ &
%   $0.000\ {\scriptstyle (0.000)}$ &
%   $0.000\ {\scriptstyle (0.000)}$ &
%   $0.000\ {\scriptstyle (0.000)}$
%   \\
% UniQA$_{BERT}$ &
%   $0.000\ {\scriptstyle (0.000)}$ &
%   $0.000\ {\scriptstyle (0.000)}$ &
%   $0.000\ {\scriptstyle (0.000)}$ 
%   \\ \hline
% \end{tabular}%
% % }
% % \caption{Performance on MIMICSQL* natural questions with evaluated with logic form accuracy ($Acc_{LF}$), execution accuracy ($Acc_{EX}$), and the structural accuracy ($Acc_{ST}$). The best in each model is in bold.}
% \label{tab:my-table}
% \vspace{-5mm}
% \end{table}

\begin{table*}[h]
\vspace{-4mm}
\centering
% \resizebox{0.5\textwidth}{%
\scriptsize
\begin{tabular}{lllllll}
\hline
{\textbf{Method}} &
  \multicolumn{3}{c}{\textbf{original}} &
  \multicolumn{3}{c}{\textbf{noise-moderate}} \\
 &
  \multicolumn{1}{c}{$Acc_{LF}$} &
  \multicolumn{1}{c}{$Acc_{EX}$} & 
  \multicolumn{1}{c}{$Acc_{ST}$} &
  \multicolumn{1}{c}{$Acc_{LF}$} &
  \multicolumn{1}{c}{$Acc_{EX}$} &
  \multicolumn{1}{c}{$Acc_{ST}$} \\ \hline
UniQA$_{BioBERT}$ &
  $0.853\ {\scriptstyle (0.008)}$ &
  $0.897\ {\scriptstyle (0.008)}$ &
  $0.901\ {\scriptstyle (0.006)}$ &
  $0.636\ {\scriptstyle (0.010)}$ &
  $\textbf{0.720}\ {\scriptstyle (0.007)}$ &
  $\textbf{0.797}\ {\scriptstyle (0.009)}$ 
  \\
UniQA$_{BlueBERT}$ &
  $\textbf{0.874}\ {\scriptstyle (0.009)}$ &
  $\textbf{0.903}\ {\scriptstyle (0.008)}$ &
  $\textbf{0.911}\ {\scriptstyle (0.011)}$ &
  $\textbf{0.668}\ {\scriptstyle (0.019)}$ &
  $0.717\ {\scriptstyle (0.021)}$ &
  $0.780\ {\scriptstyle (0.019)}$
  \\
UniQA$_{BERT}$ &
  $0.849\ {\scriptstyle (0.011)}$ &
  $0.895\ {\scriptstyle (0.009)}$ &
  $0.905\ {\scriptstyle (0.013)}$ &
  $0.610\ {\scriptstyle (0.035)}$ &
  $0.691\ {\scriptstyle (0.028)}$ &
  $0.784\ {\scriptstyle (0.028)}$
  \\ \hline
\textbf{After Recovering} \\
UniQA$_{BioBERT}$ &
  $0.879\ {\scriptstyle (0.005)}$ &
  $0.930\ {\scriptstyle (0.004)}$ &
  $0.901\ {\scriptstyle (0.006)}$ &
  $\textbf{0.731}\ {\scriptstyle (0.010)}$ &
  $\textbf{0.816}\ {\scriptstyle (0.008)}$ &
  $\textbf{0.797}\ {\scriptstyle (0.009)}$
  \\
UniQA$_{BlueBERT}$ &
  $\textbf{0.891}\ {\scriptstyle (0.009)}$ &
  $0.927\ {\scriptstyle (0.008)}$ &
  $\textbf{0.911}\ {\scriptstyle (0.011)}$ &
  $0.714\ {\scriptstyle (0.019)}$ &
  $0.768\ {\scriptstyle (0.020)}$ &
  $0.780\ {\scriptstyle (0.019)}$
  \\
UniQA$_{BERT}$ &
  $0.882\ {\scriptstyle (0.012)}$ &
  $\textbf{0.934}\ {\scriptstyle (0.008)}$ &
  $0.905\ {\scriptstyle (0.013)}$ &
  $0.695\ {\scriptstyle (0.028)}$ &
  $0.775\ {\scriptstyle (0.023)}$ &
  $0.784\ {\scriptstyle (0.028)}$
  \\ \hline
\end{tabular}%
% }
\vspace{-1mm}
\caption{Results on the \textit{test} set of MIMICSQL* and its noisy variant (\textit{i.e.} noise-moderate)}
\label{tab:biomedical_plms}
\end{table*}
